# Supplementary material for: Breaking the energy-symmetry blockade in magneto-optical rotation
Source: arXiv:1804.07522 source file (2018-04-20)
Supplement: Supplementary file 1 [file supplements20180418.pdf]

## Supplementary Material

We first emphasize that the purpose of the present work is **not** to demonstrate better than $fT/\sqrt{Hz}$ performance in magnetic field sensitivity. Such a high detection sensitivity requires a state-of-the-art magnetic shield and precision zero-field compensation measures in addition to complex RF phase-locking electronics. Our purpose is to demonstrate new physics which could potentially improve magnetometry. If we can show the superior performance with a clearly-demonstrated performance trend when comparing with a well-established single-beam $\Lambda-$scheme atomic magnetometer technology (which has been demonstrated to have $fT/\sqrt{Hz}$ sensitivity), then it is reasonable to postulate that the large enhancement effect will occur when the state-of-the-art shield and electronics are employed. This is the objective of the present work and the reasons behind the measurements shown in Fig. 1(d) and Fig. 2. In the following we provide more details on the experimental and theoretical aspects of the new technique presented in this work.

**Perturbation analysis.** Substituting the interaction Hamiltonian Eq. (1) into the Liouville equation (2) we obtain a set of equations of motion for the atomic density matrix elements $\rho_{ij} = \langle i|\hat{\rho}|j\rangle$ $(i,j = 1,..,4)$. The most relevant equations of motion to our perturbation treatment in the thin medium limit are given by $(m = 2,4)$ [34]

$$i\frac{\partial \rho_{m1}}{\partial t} = (-\delta_m - i\gamma_{m1})\rho_{m1} - \Omega_{m1}\rho_{11} - \Omega_{m3}\rho_{31}, \quad \text{(1a)}$$

$$i\frac{\partial \rho_{m3}}{\partial t} = (-\delta_2 + i\gamma_{m3})\rho_{m3} - \Omega_{3m}\rho_{11} - \rho_{13}\Omega_{m1}, \quad \text{(1b)}$$

$$i\frac{\partial \rho_{31}}{\partial t} = (-2\delta_B - i\gamma_{31})\rho_{31} - \Omega_{32}\rho_{21} - \Omega_{34}\rho_{41} + \rho_{32}\Omega_{21} + \rho_{34}\Omega_{41}. \quad \text{(1c)}$$

The corresponding equations of motion for diagonal elements $\rho_{ii}$ $(i = 1, ..., 4)$ can be derived similarly. Here, we have taken $\delta_3 = -\delta_1 \equiv \delta_B$ which is much smaller in comparison with the one-photon laser detunings $\delta_2$ and $\delta_4$.

For weak-field and large one-photon detunings Eqs. 4a-4c can be solved adiabatically by using standard perturbation theory. Taking $\Omega_{ij} = \lambda\Omega_{ij}^{(1)}$ and $\rho_{ij} = \sum_{s=0}^{\infty}\lambda^s\rho_{ij}^{(s)}$ where $\lambda$ is the perturbation order parameter, in the steady-state limit we arrive at a set of third-order solutions as the source terms describing the electric field dynamics $(m = 2,4)$,

$$\rho_{m1}^{(3)} \approx \frac{2i\rho_{11}^{(0)}\Omega_{m3}^{(1)}}{(2\delta_B + i\gamma_{31})(\delta_m + i\gamma_{m1})}\Delta_{31}, \quad \text{(2a)}$$

$$\rho_{m3}^{(3)} \approx \frac{-2i\rho_{11}^{(0)}\Omega_{m1}^{(1)}}{(2\delta_B - i\gamma_{31})(\delta_m + i\gamma_{m1})}\Delta_{13}, \quad \text{(2b)}$$

where

$$\Delta_{pq} = \sum_{j=2,4}\frac{\gamma_{j1}\Omega_{pj}^{(1)}\Omega_{jq}^{(1)}}{(\delta_j^2 + \gamma_{j1}^2)}, \quad (p,q = 1,3; p \neq q).$$

The second-order Zeeman coherence can be similarly obtained as

$$\rho_{31}^{(2)} \approx -\frac{2i\rho_{11}^{(0)}}{2\delta_B + i\gamma_{31}}\Delta_{31}. \quad \text{(3)}$$

In deriving Eqs. (5,6) we have assumed $\rho_{11}^{(0)} = \rho_{33}^{(0)} = 0.5$, $\rho_{22} = \rho_{44} = \rho_{24} = 0$, and $\rho_{2j}^{(2)} = \rho_{4j}^{(2)} = 0$ $(j = 1,3)$, in accord with perturbation assumptions in the thin-medium limit.

**NMOR effect.** Substituting Eqs. (5,6) into Eqs. (3a,3b), we obtain the numerical solution of $\mathcal{E}_p^{(\pm)}(z)$ and $\mathcal{E}_{\text{WM}}^{(\pm)}(z)$ under the steady-state approximation from which the Stokes parameters, the probe polarization rotation $\alpha$ and ellipsometry $\epsilon$ can be calculated [19]

$$S_0 = |\mathcal{E}_x^{(p)}|^2 + |\mathcal{E}_y^{(p)}|^2 = I, \quad \text{(4a)}$$

$$S_1 = |\mathcal{E}_x^{(p)}|^2 - |\mathcal{E}_y^{(p)}|^2 = Ip\cos 2\alpha\cos 2\epsilon, \quad \text{(4b)}$$

$$S_2 = 2\text{Re}(\mathcal{E}_x^{(p)}\mathcal{E}_y^{(p)*}) = Ip\sin 2\alpha\cos 2\epsilon, \quad \text{(4c)}$$

$$S_3 = -2\text{Im}(\mathcal{E}_x^{(p)}\mathcal{E}_y^{(p)*}) = Ip\sin 2\epsilon. \quad \text{(4d)}$$

where

$$p = \frac{\sqrt{S_1^2 + S_2^2 + S_3^2}}{S_0}, \quad \text{(5a)}$$

$$\alpha = \frac{1}{2}\arctan\frac{S_2}{S_1}, \quad \text{(5b)}$$

$$\epsilon = \frac{1}{2}\arctan\frac{S_3}{\sqrt{S_1^2 + S_2^2}}. \quad \text{(5c)}$$

Here, the electric field components can be obtained according to the relation $\mathcal{E}_x^{(p)} = (\mathcal{E}_p^{(+)} + \mathcal{E}_p^{(-)})/\sqrt{2}$ and $\mathcal{E}_y^{(p)} = i(\mathcal{E}_p^{(+)} - \mathcal{E}_p^{(-)})/\sqrt{2}$.

**Numerical calculations.** In numerical calculations we integrate Eqs. (2,3) without any approximations other than the usual rotating-wave approximation. This procedure yields full and rigorous electric field propagation dynamics for all four circularly-polarized field components. The results are then used to evaluate all magneto-optical parameters according to Eqs. (7,8). Figures 2-4 are obtained using this method. Parameters used in numerical calculations are $\Omega_{21}(0) = \Omega_{23}(0) = 2\pi \times 200$ kHz with $\delta_p = -2\pi\times5$ GHz and $\Omega_{41}(L) = \Omega_{43}(L) = 2\pi \times 100$ kHz with $\delta_{\text{WM}} = -2\pi\times2$ GHz. The atomic relaxation rates are chosen as $\gamma_{31} = 2\pi \times 10$ Hz and $\gamma_{21} = \gamma_{23} = \gamma_{41} = \gamma_{43} = 2\pi \times 300$ MHz (to approximate the Doppler broadened excited states). In addition, the atom density $\mathcal{N}_a = 10^{12}/\text{cm}^3$, and medium length is $L = 5$ cm.

**Experimental aspects.** We use isotopically pure $^{87}$Rb atoms as the working medium. The atomic vapor is

sealed in a cylindrical glass cell that is also filled with 933 Pa of Neon buffer gas. The uncoated cell is 5 cm in length and 2 cm in diameter. The beam diameters for the probe and WM fields are 1.8 mm and 5 mm full-width-at-half-maximum (FWHM), respectively. The atomic vapor cell is surrounded by a solenoid that was previously calibrated using two-photon spectroscopy (see Fig. S1 for birds view of the experiment layout). We employed a simple home-made magnetic field shield where two layers of magnetic alloy with high permeability form a cylindrically shaped housing (30 cm in length and 12 cm in inner diameter). The shield limit is $\simeq$ 500 nT (corresponds $\delta_B \simeq 3$ kHz) in CW operation. The temperature of the cell is maintained via convection of hot air and the typical operational temperature is 311 K to 313 K (38 $^{oo}$C to 40 $^{oo}$C). As shown in Fig. 1(c) the probe field couples the $5S_{1/2}$, $F=2$ ground state manifold to the $5P_{1/2}$, $F^{'}=1$ manifold of the $D_1$ line with a detuning of $\delta_p/2\pi=-5$ GHz. The WM field couples the $5S_{1/2}$, $F=2$ ground state manifold to the $5P_{1/2}$, $F^{'}=1$ manifold of the $D_1$ line with a detuning of $\delta_{WM}/2\pi=-2$ GHz. Typical probe and WM field intensities are 250 $\mu$W/cm$^2$ and 40 $\mu$W/cm$^2$, respectively. We do not optically pump the non-accessed $F=1$ ground-state manifold. Under these conditions we have achieved more than 300,000-fold NMOR optical signal power spectral density SNR without employing hyperfine state optical pumping. This indicates more than 550-fold NMOR optical SNR enhancement over the conventional single beam $\Lambda$ method under equal probe power and detuning. When the non-accessed hyperfine states were optically pumped we observed an additional >2 fold NMOR signal amplitude increase in time domain, bringing the observed NMOR optical SNR enhancement to over three orders of magnitude (or NMOR signal optical power spectral density $>10^6$). We emphasize that all these are achieved using a simple home-made magnetic shield and 40 Hz magnetic field modulation. With a state-of-the-art magnetic shield and RF phase-locking electronics the detection limit could be substantially further improved.

**Additional numerical results.** The propagation dynamics of the probe field is shown in Fig. S2 for the optical WM technique and the conventional single beam $\Lambda$ technique. The nonlinear $L-$dependent growth characteristics for the optical WM method [Fig. S2(a)] and the linear $L-$dependent characteristics of the conventional single-beam $\Lambda$ method restricted by the energy-symmetry NMOR blockade [Fig. S2(b)] agree well with the intuitive physical picture and experimental data given in the article

It is critically important to understand that the underlying physical principle is a deep-inelastic WM and scattering process rather than the usual double$-\Lambda$ WM process. The conventional double$-\Lambda$ WM process is cyclic in nature in field change where the gain(loss) of one circular component of the WM field must accompany the loss(gain) of the other circular component of the WM field. This cyclic transition also occurs for the probe field that is a part of the conventional cyclic double$-\Lambda$ WM process. The inelastic optical WM enhanced NMOR effect does not have this characteristics. Figure S3 shows that both circularly-polarized components of the WM drop quickly, clearly indication of the total energy loss of the WM field by an inelastic scattering process. It is at this stage the energy-symmetry NMOR blockade to the probe field is broken, unleashing the full propagation strength of the NMOR effect.

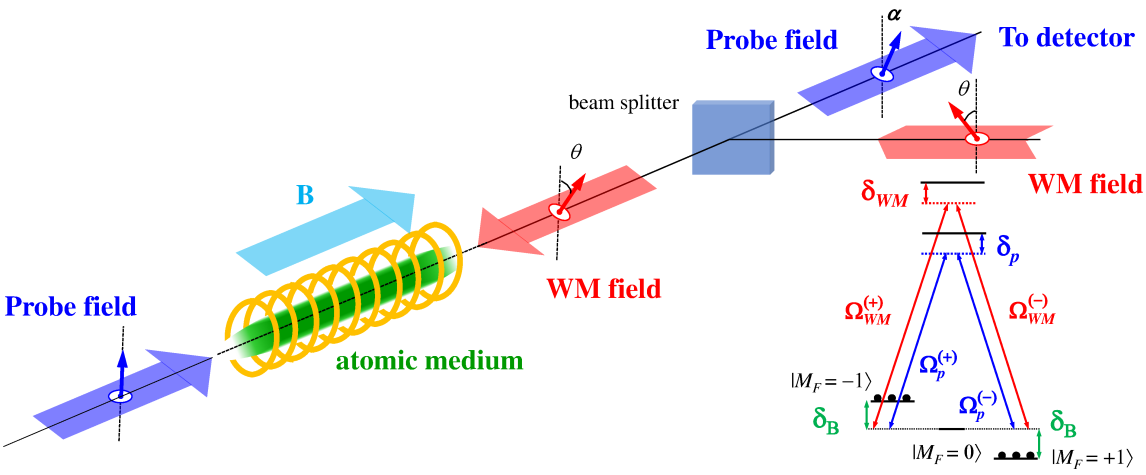


FIG. S1. Experimental schematic for the symmetry-breaking NMOR effect by optical inelastic wave mixing and scattering technique. A weak countering-propagating linearly-polarized WM field breaks the probe NMOR energy-symmetry blockade, resulting in a highly efficient NMOR by inelastic WM and scattering process.

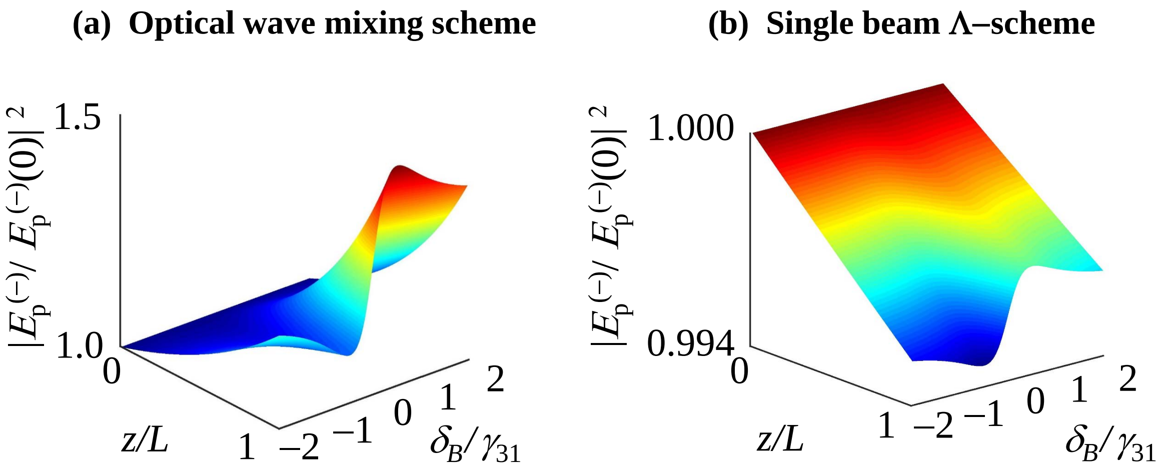


FIG. S2. Normalized intensities of the probe circularly-polarized components as functions of the normalized Zeeman shift $\delta_B/\gamma_{31}$ and propagation distance $z/L$. The nonlinear growth (a) and self-limited linear $z/L-$dependency (b) are seen. Parameters are the same as in Fig. 3 in the article.

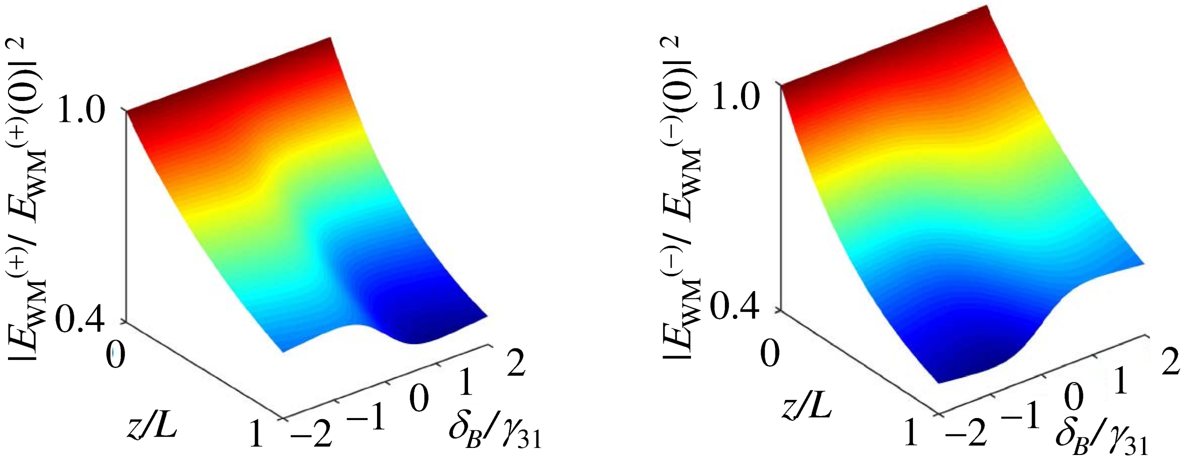


FIG. S3. Normalized intensities of the WM field circularly-polarized components as functions of the normalized Zeeman shift $\delta_B/\gamma_{31}$ and propagation distance $z/L$. The nonlinear energy loss occurs in both components indicating energy transfer by inelastic scattering from the WM field to the probe field as well as to the ground-state Zeeman coherence. Parameters are the same as in Fig. 3 in the article.
